# Supplementary material for: EdgeGaussians -- 3D Edge Mapping via Gaussian Splatting
Source: arXiv:2409.12886 source file (2025-02-11)
Supplement: Supplementary file 1 [file suppmat.tex]

% \documentclass[10pt,twocolumn,letterpaper]{article}

% \usepackage{wacv}
% \usepackage{graphicx}
% \usepackage{amsmath}
% \usepackage{amssymb}
% \usepackage{booktabs}
% \usepackage[accsupp]{axessibility}
% \input{preamble}


% \usepackage[pagebackref,breaklinks,colorlinks]{hyperref}


% \usepackage[capitalize]{cleveref}
% \crefname{section}{Sec.}{Secs.}
% \Crefname{section}{Section}{Sections}
% \Crefname{table}{Table}{Tables}
% \crefname{table}{Tab.}{Tabs.}


% \begin{document}


% % \end{figure*}\bigskip}% 

% \title{EdgeGaussians - 3D Edge Mapping via Gaussian Splatting \\
% Supplementary Material}

% \author{
% Kunal Chelani$^1$ \qquad
% %\and
% Assia Benbihi$^2$ \qquad
% %\and
% Torsten Sattler$^2$ \qquad
% %\and
% Fredrik Kahl$^1$\\
% %\and
% $^1$Chalmers University of Technology\\
% $^2$Czech Institute of Informatics, Robotics and Cybernetics, Czech Technical University in Prague\\
% {\tt\small chelani@chalmers.se}
% }

% \maketitle

% \appendix

% \cref{sec:add_imp} provides implementation details about the training of the edge-specialized Gaussian Splatting.
% \cref{sec:qual} shows qualitative results over the scenes from the  Replica~\cite{replica19arxiv} dataset used by the authors of EMAP~\cite{Li2024CVPR} and three scenes from the Tanks and Temples dataset~\cite{Knapitsch2017}.
% \cref{sec:limitations} discusses some limitations and failure cases of our method, pointing to relevant future work.


% \section{Implementation details}\label{sec:add_imp}

% \PAR{Initialization.}
% \textit{Gaussian Position:}
% For scenes from the DTU~\cite{jensen2014large}, Replica~\cite{replica19arxiv} and Tanks and Temples~\cite{Knapitsch2017} datasets, we use the SfM~\cite{schonberger2016structure} points as initialization.
% Note that random point initialization also produces reasonable, but slightly worse results.
% For \textit{ABC-NEF}~\cite{Ye_2023_CVPR}, we initialize our method with Gaussians centered at 10000 points randomly sampled in a unit cube.
% This is because the dataset comprises texture-less objects for which \gls{sfm}~\cite{schonberger2016structure} generates extremely sparse or no point reconstruction at all.
% \textit{Gaussian Scale}: We use a constant initial value of 0.004 %
% for all datasets. However, a point-dependent value based on the complexity of the neighboring region may be more robust. 
% \textit{Gaussian Opacity}: We use a constant initial value of 0.08 %
% for all datasets.
% \textit{Gaussian Orientation}: Random unit quaternions are used as initial values for all Gaussians.

% \PAR{Training.}
% We train the model for 500 epochs.
% For the first 30 epochs, we only train the position parameters so that the scale and the orientation of the Gaussian do not compensate for its incorrect position during rendering.
% Thus the training constrains the Gaussian's position, \ie, its mean, to lie on 3D edges.
% We cull the Gaussians based on opacity and duplicate the ones with high positional gradients at regular intervals as in the original work~\cite{kerbl3Dgaussians}.
% The learning rates of different parameters are as follows.
% Position: starting with $1e^{-3}$, scaled with a factor of 0.75 every 10 epochs, 5 times.
% Scale: $2e^{-4}$ constant.
% Opacity: $3e^{-2}$ constant.
% Orientation: $1e^{-3}$ constant.

% We use $k=4$ as the number of nearest neighbors for computing $\mathcal{L}_{\text{orient}}$ defined in Eq.(4) of the main paper.
% The weights of the loss function in Eq.(6) of the main paper are
% $\lambda_{1} = 0.1$ and $\lambda_{2} = 0.1$ for object level scenes from 
% \textit{ABC-NEF}~\cite{Ye_2023_CVPR} and DTU~\cite{jensen2014large}, while for larger scenes we use smaller values of $\lambda_{1} = 0.01$ and $\lambda_{2} = 0.01$.
% The geometric regularization assumes that the Gaussians are already positioned close to the edges, therefore we start applying this regularization at epoch 300.
% Note that the computation of nearest neighbors, required for the geometric regularization is computationally intensive and we observe that it is sufficient to only apply this regularization once in every 10 steps of the training process.

% \PAR{Clustering}
% During clustering, the alignment threshold is $\theta = 0.8$ on \textit{ABC-NEF}~\cite{Ye_2023_CVPR}, which have clean straight lines, and $\theta = 0.6$ on DTU~\cite{jensen2014large} to account for the higher curvature of the shapes.
% During the parametric edge fitting, we fit a curve whenever the curve residual error is $\delta = 0.5$ lower than the line residual error. For objects from the DTU dataset~\cite{jensen2014large}, due to the prior knowledge that the objects have more curves than lines, a larger $\delta = 1$ is used.

% For any further clarifications, please refer to the code released at \href{https://github.com/kunalchelani/EdgeGaussians.}{https://github.com/kunalchelani/EdgeGaussians.}


% \section{Additional Qualitative Results}\label{sec:qual}
% \cref{fig:qual_replica0} to~\ref{fig:qual_replica2} show the results for the scenes \textit{room\_0}, \textit{room\_1}, \textit{room\_2} of the Replica~\cite{replica19arxiv} dataset. 
% The results show that our method produces edges with a higher completeness than EMAP~\cite{Li2024CVPR}. 
% Also, EMAP~\cite{Li2024CVPR} predicts clusters of duplicate edges close to the ground-truth edge, which is not a desirable result 
% as it makes the reconstruction less sharp.
% Overall, our method produces clean single edges that are more complete.
% However, in some cases, EMAP~\cite{Li2024CVPR} produces geometrically accurate lines, which our method captures as incomplete curves.
% \cref{fig:qual_replica1} shows one such example.
% Although this can be partially addressed by adjusting the parameter $\delta$ involved in the model selection when fitting a line or a curve, this could be seen as a current limitation of our method.

% \section{Limitations and Failure Cases}\label{sec:limitations}
% \PAR{Fine structures and geometric regularization.}
% As briefly described in the main paper, 
% %while the geometric regularization and clustering process work well in general, there is room for improvement. Firstly, 
% the method is limited by the noise in the supervisory signal of the 2D edge maps.
% In many cases the fine structures in such edge maps~\cite{su2021pixel,poma2020dense} are not discernible, leading to incorrectly positioned edge points. 
% Geometric regularization applied to noisy edge points can lead the Gaussians' %positioning and orientation so as 
% to form short local curves to satisfy the alignment with their nearest neighbors. Examples of such cases can be seen in~\cref{fig:failure}. 

% \PAR{Clustering and edge fitting.}
% Further, the clustering algorithm exhibits limitations when applied to larger scenes with complex structures. 
% \cref{fig:qual_tnt} shows examples from the Tanks and Temples dataset~\cite{Knapitsch2017} where the oriented edge points (red), \ie, the 3D Gaussians, better cover the ground-truth 3D edges than the paramtric edges (black).
% %obtained from the optimized 3D Gaussians provide better coverage of the actual edges present in the scene. 
% One explanation is that the graph traversal based clustering removes several correct edge components close to the true scene structure while including several incorrect edges. 
% Instead of relying only on local geometric heuristics, defining a prior on which parts of the scene are more likely to hold 3D edge could improve the method's robustness.
% %can add to the robustness of the method
% %Instead of only heuristics, having a prior on which parts of the scene are more likely to contain 3D edge can add to the robustness of the method. 


% \begin{figure*}
%     \centering
%     \includegraphics[width=\linewidth]{replica_qual_room0_reduced.pdf}
%     \caption{\textbf{Replica~\cite{replica19arxiv} \textit{room\_0}} : Qualitative result showing edges produced by our method and EMAP~\cite{Li2024CVPR}. In general it can be observed that EMAP~\cite{Li2024CVPR} has several duplicate / dense sets of edges close to ground-truth edges whereas our method produces clean single edges.}
%     \label{fig:qual_replica0}
% \end{figure*}


% \begin{figure*}
%     \centering
%     \includegraphics[width=\linewidth]{replica_qual_room1_reduced.pdf}
%     \caption{\textbf{Replica~\cite{replica19arxiv} \textit{room\_1}} : Qualitative result showing three different views of edges produced by our method and EMAP~\cite{Li2024CVPR}. In general it can be observed that EMAP~\cite{Li2024CVPR} has several duplicate / dense sets of edges close to ground-truth edges, while our method produces clean single edges.
%     However, EMAP~\cite{Li2024CVPR} produces more accurate lines for some geometric edges, for example, on the window pane.}
%     \label{fig:qual_replica1}
% \end{figure*}

% \begin{figure*}
%     \centering
%     \includegraphics[width=\linewidth]{replica_qual_room2_reduced.pdf}
%     \caption{\textbf{Replica~\cite{replica19arxiv} \textit{room\_2}} : Qualitative result showing edges produced by our method and EMAP~\cite{Li2024CVPR}. In general it can be observed that EMAP~\cite{Li2024CVPR} has several duplicate / dense sets of edges close to ground-truth edges, while our method produces clean single edges.}
%     \label{fig:qual_replica2}
% \end{figure*}

% \begin{figure*}
%     \centering
%     \includegraphics[width=\linewidth]{tnt-crop.pdf}
%     \caption{\textbf{Tanks and Temples~\cite{Knapitsch2017}}: Qualitative result showing edges produced by our method on three scenes from the tanks and temples dataset. Supervisory signal (Left), edge points represented as a small line segment centered at the mean of the optimized 3D Gaussians and oriented towards their principal directions (Middle) and the points sampled on the parametric 3D edges estimated (Right). Note that the estimated Gaussians faithfully represent the scene but the clustering and edge fitting process have room for improvement 
%     %scope for robustness 
%     as many correct edges are missed and spurious ones are created in this process.}
%     \label{fig:qual_tnt}
% \end{figure*}

% \begin{figure*}
%     \centering
%     \includegraphics[width=\linewidth]{failures-crop.pdf}
%     \caption{\textbf{Failure cases} : Scans \textit{00009685}, \textit{00002412} and \textit{00003884} (left to right) on the \textit{ABC-NEF}~\cite{Ye_2023_CVPR}. 
%     The edges predicted by our method are shown in black and the ground-truth ones in green.
%     These examples are challenging because they show extremely thin structures: the projection on two distinct parallel and close 3D edges can get projected into a single edge in several views of the supervisory 2D edge maps~\cite{su2021pixel,poma2020dense}.
%     Another example where the proposed method is incomplete (right) is when the object has 3D edges inside the structure that are not detected by the 2D edge detectors.
%     Then, there is no supervisory signal for those 3D edges.
%     }
%     \label{fig:failure}
% \end{figure*}

% {\small
% \bibliographystyle{ieee_fullname}
% \bibliography{egbib}
% }


% \end{document}
